# Supplementary material for: SLING: Sino Linguistic Evaluation of Large Language Models
Source: arXiv:2210.11689 source file (2022-10-21)
Supplement: Supplementary file 1 [file appendix_old.tex]

\section{Appendix}

\subsection{Alternative Question}

% \begin{exe}
%     \exi{(8)}
%     \begin{xlist}
%     \ex \gll tamen shi qiantai haishi mujiang?\\
%         they are receptionist or carpenter\\
%         \glt ``Are they receptionists or carpenters?"
        
%     \ex[*]{\gll tamen shi qiantai haishi mujiang \textbf{ma}?\\
%         they are receptionist or carpenter \texttt{SP}\\}
%     \end{xlist}
% \end{exe}

\begin{table*}[!h]
\centering
\resizebox{\textwidth}{!}{%
\begin{tabular}{@{}lcccccccc@{}}
\toprule
      & Min. & 1st. Qu & Median & Mean  & 3rd. Qu & Max. & SD       & Shapiro-Wilk Normality Test  \\ \midrule
Mono  & 47.4 & 74.95   & 82.5   & 79.78 & 90.62   & 94.3 & 15.293 & $W = 0.863$, $p = 0.130$ \\
Multi & 6.5  & 18.1    & 45.3   & 36.16 & 54.1    & 56.9 & 21.653 & $W = 0.847$, $p = 0.116$ \\ \bottomrule
\end{tabular}%
}
\caption{Basic statistics of the accuracies of the mono- and multi-lingual LMs on the alternative question phenomenon. A minimal pair example is given in (\ref{ex.altq}). \yscomment{maybe delete this since bar plot obvious}}
\label{tab:AltQbasicstats}
\end{table*}


\begin{figure*}[!h]
\centering
\resizebox{\textwidth}{!}{%
\includegraphics{figs/AltQ.pdf}%
}
\caption{The accuracies of the LMs on the alternative question phenomenon.}
\label{fig.altq}
\end{figure*}
% https://colab.research.google.com/drive/1yPOKeFYeyIlsWJ3ihFstGpBha3GmzGZY?usp=sharing

\subsection{Anaphor (Gender)}

%%% Anaphor Male %%%

\begin{table*}[!h]
\centering
\resizebox{\textwidth}{!}{%
\begin{tabular}{llccccccc}
\toprule
      & Min.  & 1st. Qu & Median & Mean  & 3rd. Qu & Max. & SD     & Shapiro-Wilk Normality Test \\ \midrule
Mono  & 2.6   & 48.17   & 50.8   & 51.64 & 59.2    & 87.6 & 24.817 & $W = 0.899$, $p = 0.283$    \\
Multi & 16.30 & 27.8    & 38.30  & 51.47 & 78.20   & 93.7 & 31.011 & $W = 0.882$, $p = 0.238$    \\ \bottomrule
\end{tabular}%
}
\caption{Basic statistics of the accuracies of the mono- and multi-lingual LMs on the male gender baseline (Male Baseline) in the anaphor phenomenon. A minimal pair example is given in (\ref{ex.current.binding}).}
\label{tab:malebaselinemonomulti}
\end{table*}


\begin{table*}[!h]
\centering
\resizebox{\textwidth}{!}{%
\begin{tabular}{llccccccc}
\toprule
      & Min.  & 1st. Qu & Median & Mean  & 3rd. Qu & Max.  & SD      & Shapiro-Wilk Normality Test \\ \midrule
Mono  & 7.60  & 75.10   & 88.25  & 76.72 & 94.17   & 99.60 & 30.917 & $W = 0.750$, $p = 0.008$    \\
Multi & 10.50 & 37.60   & 48.60    & 50.71 & 60.55   & 99.60   & 28.06  & $W = 0.962$, $p = 0.839$    \\ \bottomrule
\end{tabular}%
}
\caption{Basic statistics of the accuracies of the mono- and multi-lingual LMs on the male anaphor gender agreement (Male Self) in the anaphor phenomenon. A minimal pair example is given in (\ref{ex.current.binding.reflexive}).}
\label{tab:maleppmonomulti}
\end{table*}


\begin{table*}[!h]
\centering
\resizebox{\textwidth}{!}{%
\begin{tabular}{llccccccc}
\toprule
      & Min.   & 1st. Qu & Median & Mean  & 3rd. Qu & Max.  & SD      & Shapiro-Wilk Normality Test \\ \midrule
Mono  & 16.20  & 39.23  & 56.55  & 58.14 & 79.62   & 91.60 & 28.12   & $W = 0.905$, $p = 0.318$    \\
Multi & 13.90  & 20.00  & 28.70  & 32.26 & 35.85   & 71.50   & 19.48 & $W = 0.852$, $p = 0.128$    \\ \bottomrule
\end{tabular}%
}
\caption{Basic statistics of the accuracies of the mono- and multi-lingual LMs on the male anaphor gender agreement with a \texttt{PP} (Male Self PP) in the anaphor phenomenon. A minimal pair example is given in (\ref{ex.current.binding.reflexive}).}
\label{tab:maleselfmonomulti}
\end{table*}


\begin{table*}[!h]
\centering
\resizebox{\textwidth}{!}{%
\begin{tabular}{llccccccc}
\hline
      & Min.  & 1st. Qu & Median & Mean  & 3rd. Qu & Max.  & SD     & Shapiro-Wilk Normality Test \\ \hline
Mono  & 80.20 & 85.53   & 90.25  & 89.26 & 92.12   & 96.40 & 5.365  & $W = 0.963$, $p = 0.835$    \\
Multi & 39.20 & 44.30   & 62.80  & 61.13 & 73.40   & 90.50 & 20.075 & $W = 0.914$, $p = 0.424$    \\ \hline
\end{tabular}%
}
\caption{Basic statistics of the accuracies of the mono- and multi-lingual LMs on the female gender baseline (Female Baseline) in the anaphor phenomenon.}
\label{tab:femalebaselinemonomulti}
\end{table*}

\begin{table*}[!h]
\centering
\resizebox{\textwidth}{!}{%
\begin{tabular}{llccccccc}
\toprule
      & Min.  & 1st. Qu & Median & Mean  & 3rd. Qu & Max.  & SD     & Shapiro-Wilk Normality Test \\ \midrule
Mono  & 80.80 & 92.90   & 96.80  & 94.47 & 98.58   & 99.70 & 6.447  & $W = 0.819$, $p = 0.045$    \\
Multi & 44.00 & 54.20   & 71.00  & 69.84 & 83.65   & 98.20 & 20.159 & $W = 0.949$, $p = 0.772$    \\ \bottomrule
\end{tabular}%
}
\caption{Basic statistics of the accuracies of the mono- and multi-lingual LMs on the female anaphor gender agreement (Female Self) in the anaphor phenomenon.}
\label{tab:femaleselfmonomulti}
\end{table*}

\begin{table*}[!h]
\centering
\resizebox{\textwidth}{!}{%
\begin{tabular}{llccccccc}
\toprule
      & Min.  & 1st. Qu & Median & Mean  & 3rd. Qu & Max.  & SD     & Shapiro-Wilk Normality Test \\ \midrule
Mono  & 26.90 & 65.47   & 73.35  & 71.19 & 84.30   & 95.40 & 20.93558  & $W = .88488$, $p = 0.2096$    \\
Multi & 18.90 & 50.55   & 71.60  & 65.91 & 86.15   & 97.50 & 30.24905 & $W = 0.88144$, $p = 0.2329$    \\ \bottomrule
\end{tabular}%
}
\caption{Basic statistics of the accuracies of the mono- and multi-lingual LMs on the female anaphor gender agreement with a \texttt{PP} (Female Self PP) in the anaphor phenomenon.}
\label{tab:femaleppmonomulti}
\end{table*}



%%% Male Baseline Self Mono Wilcox %%%

\begin{table*}[!h]
\centering
\resizebox{0.75\linewidth}{!}{%
\begin{tabular}{|l|cccc|c|c|}
\hline
\multicolumn{1}{|c|}{\multirow{2}{*}{\textit{Pair}}} & \multicolumn{4}{c|}{Paired Differences}                                                                                                                                & \multirow{2}{*}{\textit{Z}} & \multirow{2}{*}{\textit{p}} \\ \cline{2-5}
\multicolumn{1}{|c|}{}                               & \multicolumn{1}{c|}{Mean}                    & \multicolumn{1}{c|}{Median}                 & \multicolumn{1}{c|}{SD}                     & \textit{n} &                             &                             \\ \hline
Male Baseline Mono                                   & \multicolumn{1}{c|}{\multirow{2}{*}{-25.09}} & \multicolumn{1}{c|}{\multirow{2}{*}{-27.8}} & \multicolumn{1}{c|}{\multirow{2}{*}{16.97}} & \multirow{2}{*}{8}          & \multirow{2}{*}{0.94}       & \multirow{2}{*}{0.008}      \\ \cline{1-1}
Male Self Mono                                       & \multicolumn{1}{c|}{}                        & \multicolumn{1}{c|}{}                       & \multicolumn{1}{c|}{}                       &                             &                             &                             \\ \hline
\end{tabular}%
}
\caption{A two-sided paired Wilcoxon signed rank exact test was conducted to compare the performance of the mono-lingual LMs on the Male Baseline and Male Self paradigms. There was a significant difference in the accuracies of the Male Baseline (mean = $51.64$, median = $50.8$, SD = $24.817$) and the Male Self (mean = $76.72$, median = $88.25$, SD = $30.917$); $Z = 0.94$, $p = 0.008$.}
\label{tab:male.mono.baseline.self}
\end{table*}

%%% Male Baseline Self Multi %%%

\begin{table*}[!h]
\centering
\resizebox{0.75\linewidth}{!}{%
\begin{tabular}{|l|cccc|c|c|}
\hline
\multicolumn{1}{|c|}{\multirow{2}{*}{Pair}} & \multicolumn{4}{c|}{Paired Differences}                                                                                        & \multirow{2}{*}{t(7)} & \multirow{2}{*}{p}    \\ \cline{2-5}
\multicolumn{1}{|c|}{}                               & \multicolumn{1}{c|}{Mean}                  & \multicolumn{1}{c|}{SD}                     & \multicolumn{2}{c|}{95\% CI}        &                       &                       \\ \hline
Male Baseline Multi                                  & \multicolumn{1}{c|}{\multirow{2}{*}{0.76}} & \multicolumn{1}{c|}{\multirow{2}{*}{25.32}} & \multicolumn{1}{c|}{Lower}  & Upper & \multirow{2}{*}{0.08} & \multirow{2}{*}{0.94} \\ \cline{1-1} \cline{4-5}
Male Self Multi                                      & \multicolumn{1}{c|}{}                      & \multicolumn{1}{c|}{}                       & \multicolumn{1}{c|}{-22.66} & 24.17 &                       &                       \\ \hline
\end{tabular}%
}
\caption{A two-sided paired t-test was conducted to compare the performance of the multi-lingual LMs on the Male Baseline and Male Self paradigms. There was no significant difference in the accuracies of the Male Baseline (mean = $51.47$, SD = $31.01$) and the Male Self (mean = $50.71$, SD = $28.06$); $t\text{(7)} = 0.08$, $p = 0.94$.}
\label{tab:male.multi.baseline.self}
\end{table*}

%%% Male Baseline & PP Mono %%%
% If the LMs even only know a tiny bit about hierarchy, the performance of PP should be better than Baseline.

%%% Male Baseline & PP Multi %%%

%%% Female Baseline vs. Female Self Mono%%%

\begin{table*}[!h]
\centering
\resizebox{0.75\linewidth}{!}{%
\begin{tabular}{|l|clcc|c|c|}
\hline
\multicolumn{1}{|c|}{\multirow{2}{*}{\textit{Pair}}} & \multicolumn{4}{c|}{Paired Differences}                                                                                                                    & \multirow{2}{*}{\textit{Z}} & \multirow{2}{*}{p}    \\ \cline{2-5}
\multicolumn{1}{|c|}{}                               & \multicolumn{1}{c|}{Mean}                   & \multicolumn{1}{c|}{Median}                & \multicolumn{1}{c|}{SD}                    & \textit{n}                  &                             &                       \\ \hline
Female Baseline Mono                                  & \multicolumn{1}{c|}{\multirow{2}{*}{-5.21}} & \multicolumn{1}{c|}{\multirow{2}{*}{-5.1}} & \multicolumn{1}{c|}{\multirow{2}{*}{5.54}} & \multirow{2}{*}{8} & \multirow{2}{*}{0.62}       & \multirow{2}{*}{0.08} \\ \cline{1-1}
Female Self Mono                                      & \multicolumn{1}{c|}{}                       & \multicolumn{1}{l|}{}                      & \multicolumn{1}{c|}{}                      &                    &                             &                       \\ \hline
\end{tabular}%
}
\caption{A two-sided paired Wilcoxon signed rank exact test was conducted to compare the performance of the mono-lingual LMs on the Female Baseline and Female Self paradigms. There was no significant difference in the accuracies of the Female Baseline (mean = $89.26$, median = $90.25$, SD = $5.36$) and the Female Self (mean = $94.47$, median = $96.80$,SD = $6.45$); \textit{Z} = $0.62$, $p = 0.08$.}
\label{tab:female.mono.baseline.self}
\end{table*}


%%% Female Baseline Self Multi %%%

\begin{table*}[!h]
\centering
\resizebox{0.75\linewidth}{!}{%
\begin{tabular}{|l|cccc|c|c|}
\hline
\multicolumn{1}{|c|}{\multirow{2}{*}{Pair}} & \multicolumn{4}{c|}{Paired Differences}                                                                                        & \multirow{2}{*}{\textit{t(7)}} & \multirow{2}{*}{\textit{p}} \\ \cline{2-5}
\multicolumn{1}{|c|}{}                      & \multicolumn{1}{c|}{Mean}                   & \multicolumn{1}{c|}{SD}                    & \multicolumn{2}{c|}{95\% CI}        &                                &                             \\ \hline
Female Baseline Multi                       & \multicolumn{1}{c|}{\multirow{2}{*}{-8.71}} & \multicolumn{1}{c|}{\multirow{2}{*}{9.30}} & \multicolumn{1}{c|}{Lower}  & Upper & \multirow{2}{*}{-2.48}         & \multirow{2}{*}{0.048}      \\ \cline{1-1} \cline{4-5}
Female Self Multi                           & \multicolumn{1}{c|}{}                       & \multicolumn{1}{c|}{}                      & \multicolumn{1}{c|}{-17.31} & -0.11 &                                &                             \\ \hline
\end{tabular}%
}
\caption{A two-sided paired t-test was conducted to compare the performance of the multi-lingual LMs on the Female Baseline and Female Self paradigms. There was a significant difference in the accuracies of the Female Baseline (mean = $61.13$, SD = $20.08$) and the Female Self (mean = $69.84$, SD = $20.16$); $t\text{(7)} = -2.48$, $p = 0.048$.}
\label{tab:female.multi.baseline.self}
\end{table*}



\begin{figure*}[!h]
\centering
\resizebox{\textwidth}{!}{%
\includegraphics{figs/AnaphorMaleBaselineSelf.png}%
}
\caption{The accuracy of the LMs on the male gender baseline (Male Baseline) and male anaphor gender agreement (Male Self) paradigms. The subject of the paradigms is male. The Male Baseline show the preference of the LMs to a male object. The Male Self show the accuracy of a model when the object gender needs to agree with the subject.}
\label{fig.male.base.self}
\end{figure*}

\begin{figure*}[!h]
\centering
\resizebox{\textwidth}{!}{%
\includegraphics{figs/AnaphorMaleSelfPP.png}%
}
\caption{The accuracy of the LMs on the male anaphor gender agreement (Male Self) and male anaphor gender agreement with a distractor (Male PP) paradigms. The subject of the paradigms is male. The Male Self show the accuracy of a model when the object gender needs to agree with the subject. The Male PP show the accuracy of a model when the object gender needs to agree with the subject with the presence of a distractor of the opposite gender.}
\label{fig.male.self.pp}
\end{figure*}

\begin{figure*}[!h]
\centering
\resizebox{\textwidth}{!}{%
\includegraphics{figs/AnaphorMaleBaselinePP.png}%
}
\caption{The accuracy of the LMs on the male gender baseline (Male Baseline) and male anaphor gender agreement with a distractor (Male PP) paradigms. The subject of the paradigms is male. The Male Baseline show the preference of the LMs to a male object. The Male PP show the accuracy of a model when the object gender needs to agree with the subject with the presence of a distractor of the opposite gender.}
\label{fig.male.baseline.pp}
\end{figure*}

%%% Anaphor Female %%%

\begin{figure*}[!h]
\centering
\resizebox{\textwidth}{!}{%
\includegraphics{figs/AnaphorFemaleBaselineSelf.png}%
}
\caption{The accuracy of the LMs on the female gender baseline (Female Baseline) and female anaphor gender agreement (Female Self) paradigms. The subject of the paradigms is female. The Female Baseline show the preference of the LMs to a female object. The Female Self show the accuracy of a model when the object gender needs to agree with the subject.}
% \label{fig.cl.comp.adj}
\end{figure*}

\begin{figure*}[!h]
\centering
\resizebox{\textwidth}{!}{%
\includegraphics{figs/AnaphorFemaleSelfPP.png}%
}
\caption{The accuracy of the LMs on the female anaphor gender agreement (Female Self) and female anaphor gender agreement with a distractor (Female Self PP) paradigms. The subject of the paradigms is female. The Female Self show the accuracy of a model when the object gender needs to agree with the subject. The Female PP show the accuracy of a model when the object gender needs to agree with the subject with the presence of a distractor of the opposite gender.}
\label{fig.female.self.pp}
\end{figure*}

\begin{figure*}[!h]
\centering
\resizebox{\textwidth}{!}{%
\includegraphics{figs/AnaphorFemaleBaselinePP.png}%
}
\caption{The accuracy of the LMs on the female gender baseline (Female Baseline) and female anaphor gender agreement with a distractor (Female PP) paradigms. The subject of the paradigms is female. The Female Baseline show the preference of the LMs to a female object. The Female PP show the accuracy of a model when the object gender needs to agree with the subject with the presence of a distractor of the opposite gender.}
\label{fig.female.baseline.pp}
\end{figure*}

%%% Aspect %%%

\begin{figure*}[!h]
\centering
\resizebox{\textwidth}{!}{%
\includegraphics{figs/AspectGuoLeInPastTense.png}%
}
\caption{The accuracy of the LMs on the knowledge that \textit{guo} and \textit{le} occur in the past tense when there is no future oriented adverbs and morphemes like \textit{cai} or \textit{jiu}. In both paradigms, the good sentences have a past oriented adverb and the bad ones have a future oriented adverb without \textit{cai} or \textit{jiu}.}
% \label{fig.cl.comp.adj}
\end{figure*}

\begin{figure*}[!h]
\centering
\resizebox{\textwidth}{!}{%
\includegraphics{figs/AspectZaiGuoLe.png}%
}
\caption{The accuracy of the LMs on the knowledge that \textit{guo} and \textit{le} do not co-occur with the progressive marker \textit{zai} when they are between a verb and its object (e.g., \textit{eat} le \textit{an apple}). In both paradigms, the good sentences have no \textit{zai} and the bad ones have.}
% \label{fig.cl.comp.adj}
\end{figure*}

\begin{figure*}[!h]
\centering
\resizebox{\textwidth}{!}{%
\includegraphics{figs/AspectZaiLeScope.png}%
}
\caption{The accuracy of the LMs on the knowledge that: i) \textit{zai} \& \textit{le} in VP --- when \textit{zai} is present, \textit{le} cannot occur between a verb and its object (e.g., \textit{eat} le \textit{an apple}); ii) \textit{zai} \& \textit{le} after VP ---  when \textit{zai} is present, \textit{le} can occur after the object of a verb.}
% \label{fig.cl.comp.adj}
\end{figure*}

%%% Definiteness Effect %%%

\begin{figure*}[!h]
\centering
\resizebox{\textwidth}{!}{%
\includegraphics{figs/DefEffect.png}%
}
\caption{The accuracy of the LMs on the knowledge that demonstratives \textit{zhe} (this) and \textit{na} (that) as well as the universal quantifier \textit{mei} (every) cannot occur after the existential \textit{you} (have), a counterpart of English \textit{there}-construction. In both paradigms, the good sentences have numeral + classifier before the noun while the bad ones have \textit{zhe}/\textit{na}/\textit{mei} before the noun.}
% \label{fig.cl.comp.adj}
\end{figure*}

%%% Polarity Item %%%

\begin{figure*}[!h]
\centering
\resizebox{\textwidth}{!}{%
\includegraphics{figs/PolarityItem.png}%
}
\caption{The accuracy of the LMs on the knowledge that: i) \textit{renhe} (any) and \textit{shenme} (what) as a polarity item occur in negative contexts but not in affirmative contexts; ii) \textit{huoduohuoshao} only occurs in affirmative contexts.}
% \label{fig.cl.comp.adj}
\end{figure*}

%%% Relative Clause %%%

\begin{figure*}[!h]
\centering
\resizebox{\textwidth}{!}{%
\includegraphics{figs/RelativeClause.png}%
}
\caption{The accuracy of the LMs on the knowledge that in simple subject relative clauses the gap should not be filled with the head noun of the relative clauses (e.g., \textit{the person who \rule{0.3cm}{0.15mm} ate the apple} vs. *\textit{the person who the person ate the apple}) or a pronoun referring to the head noun (e.g., \textit{the person who \rule{0.3cm}{0.15mm} ate the apple} vs. *\textit{the person who he/she ate the apple}).}
% \label{fig.cl.comp.adj}
\end{figure*}
